# Supplementary material for: Strain-induced alignment in collagen gels
Source: arXiv:0907.1855 source file (2009-07-10)
Supplement: Supplementary file 1 [file Supplementary.pdf]

# Validation of fiber orientation algorithm

The image processing method described in the manuscript to extract localcollagen fibril orientation from confocal images has been validated on computer-made random networks of sticks on a 2D plane. A large number of sticks of a given length are drawn at random (position and orientation) on an image (see Figure 1a) to simulate the appearance of the experimental images of collagen network. In addition, image blur and Gaussian noise have been introduced (Figure 1b). These images are then submitted to the analysis described in the paper. Figure 1c shows the local fiber orientation at every location where fiber could be non-ambiguously detected.

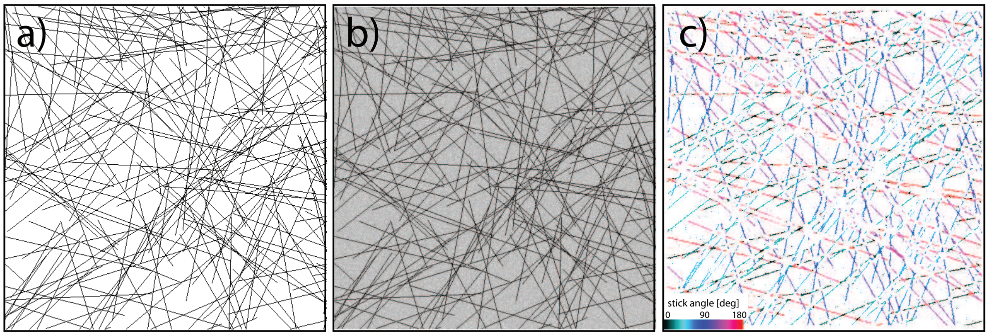


Figure 1: (a) Example of a simulated random network of sticks in two dimensions. (b) Same example, after blurring and added Gaussian noise. (c) Color-coded local stick orientation, as determined by our image processing algorithm. Angle color scale at bottom

We then compare the true histogram of stick orientations, which is calculated while the original image is created, with the angular distribution calculated by the image analysis method (Figure 2a). To determine whether the two histograms - the true one and the measured one - are from the same probability distribution, we use the Kolmogorov-Smirnov test (1), which is based on the comparison of the two cumulative probability distributions (see Figure 2b). In all validation tests conducted on simulated images of densities comparable to our confocal data, we find that the Kolmogorov-Smirnov test does not allow us to reject the null hypothesis that the two histograms are from the same probability distribution function ($p$-value $> 0.05$). In most, but not all cases, the $p$-value is even greater than 0.2; the example illustrated in Figures 1 and 2 has $p > 0.2$.

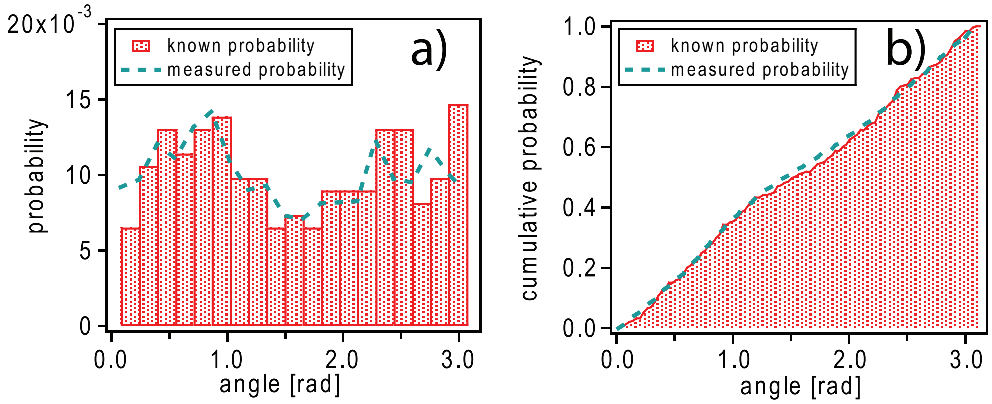


Figure 2: Known and calculated (a) probability density functions and (b) cumulative distribution functions of the orientation of individual sticks, based on image shown in Figure 1a.

## References

1. Lehmann, E. L., and J. P. Romano, 2005. Testing Statistical Hypotheses. Springer.
